# Supplementary material for: On the Limitation and Experience Replay for GNNs in Continual Learning
Source: arXiv:2302.03534 source file (2024-07-09)
Supplement: Supplementary file 1 [file appendix_additional_exp_results.tex]

\section{Additional Experimental Results}
In this appendix, we provide additional experimental results for our study. For the additional experimental result, we focus on the real-world evolving dataset, OGBN-arxiv, and mainly use average stage performance for the main metric. We provide a more detailed experimental result on how the average stage performance change along with hidden layer dimension and a more detailed study on the hyper-parameters of each component of our proposed framework.  All the experiments are done with GCN as the base module.

\subsection{Hidden Layer Dimension}
In this experiment, we provide more detailed dynamics of the performance of GNNs with respect to their hidden layer dimension in the static and continual learning setting. In this experiment, we simply train the GNNs on OGBN-arxiv in both the static setting and continual setting described above. As shown in Fig.~\ref{fig:hidden_dim}, the performance of the GNN in the static setting is much higher than the one in the continual setting. As we discussed in the main text, one of the main reasons for this is the sequential bias introduced by the continual learning setting. At each stage, the system biases toward the most current data and ``forget'' the previous data. In addition, the dynamic shows that the continual learning setting requires a higher hidden dimension due to different distributions in the process, as we discussed in the main text. 

% \begin{figure}
%     \centering
%     \includegraphics[scale=0.2]{figure/add_exp/hidden_dimension.png}
%     \caption{Average stage performance on different hidden layer dimension.}
%     \label{fig:hidden_dim}
% \end{figure}

\begin{figure}
    \centering
    \begin{minipage}{.45\textwidth}
        \centering
        \includegraphics[width=0.95\linewidth, height=0.2\textheight]{figure/add_exp/hidden_dimension.png}
         \caption{Average stage performance on \\ different hidden layer dimension.}
    \label{fig:hidden_dim}
    \end{minipage}%
    \begin{minipage}{0.45\textwidth}
        \centering
        \includegraphics[width=0.95\linewidth, height=0.2\textheight]{figure/add_exp/replay_size.png}
        \caption{Average stage performance on different replay set size.}
    \label{fig:replay_size}
    \end{minipage}
\end{figure}

\subsection{Replay Set Size}
In this experiment, we fix the hidden layer of GNNs of dimension $256$ and do not use CMD regularisation in the training. We vary the size of the replay set (with respect to \% of training set size). As shown in Fig.~\ref{fig:replay_size}, the average stage performance of the framework (with only the replay component) increases initially when we increase the replay set size. The improvement becomes insignificant after $0.05$ (even a slight decline). The reason for this could be that the training process at the new stage is initialized with parameters learnt from the previous data. This means that the model starts with a parameter that is already biased toward the previous data. A larger replay set can decreases the catastrophic forgetting of the system for the previous stage. However, this might be at the cost of bringing down the performance for newer data, as the replay set adds bias to the data from the previous stage. As a result, the average stage performance might not improve (even decrease) if the replay set size is too large. This shows that the ``optimal'' replay set size is small and replay strategy only adds a small fraction of the training cost.

\subsection{CMD Beta Value}
In this experiment, we fix the hidden layer of GNNs of dimension $256$ and do not use experience replay in the training. Recall that the loss function with CMD regularization is given as follows.
$$
    \mathcal{L} =  \mathcal{L}_c(\hat{\mathcal{V}}_i^{tr}) + \beta \text{CMD}(\mathcal{Z}_{\text{train}},\mathcal{Z}_{\text{IID}}),
$$
where $\mathcal{L}_c(\hat{\mathcal{V}}_i^{tr})$ is the classification loss from the training set, $\mathcal{Z}_{\text{train}}$ is the set of representations from the vertexes of the training set and $\mathcal{Z}_{\text{IID}}$ is the set of representations from the vertexes of the anchor set $\mathcal{I}$, which we randomly sample from the rest of vertexes. For this experiment, the size of $\mathcal{I}$ is 12.5\% (128) of the batch size (1024). We vary the value of $\beta$ in the equation above from the list $[1,5,10,100,1000]$. As shown in Fig.~\ref{fig:cmd_beta}, there is no significant difference between the performance when $\beta$ is small but there is a significant drop in the performance when $\beta$ becomes too big. $\beta$ control the regularization effect from the CMD term. If we make $\beta$ too large, the regularization term would trump the first term (classification performance). This makes the model converge to a parameter where the representations might be closed but the classification performance is poor.

\begin{figure}
    \centering
    \begin{minipage}{.45\textwidth}
        \centering
        \includegraphics[width=0.95\linewidth, height=0.2\textheight]{figure/add_exp/cmd_beta.png}
        \caption{Average stage performance on \\ different beta value.}
      \label{fig:cmd_beta}
    \end{minipage}%
    \begin{minipage}{0.45\textwidth}
        \centering
        \includegraphics[width=0.95\linewidth, height=0.2\textheight]{figure/add_exp/cmd_size.png}
        \caption{Average stage performance on \\different size of anchor set.}
    \label{fig:cmd_size}
    \end{minipage}
\end{figure}

% \begin{figure}
%     \centering
%     \includegraphics[scale=0.2]{figure/add_exp/cmd_beta.png}
%     \caption{Average stage performance on different beta value.}
%     \label{fig:cmd_beta}
% \end{figure}

% \begin{figure}
%     \centering
%     \includegraphics[scale=0.2]{figure/add_exp/cmd_size.png}
%     \caption{Average stage performance on different size of anchor set.}
%     \label{fig:cmd_size}
% \end{figure}

\subsection{CMD Anchor Set Size}
In this experiment, we fix the hidden layer of GNNs of dimension $256$ and do not use experience replay in the training. We follow a similar setting as the previous experiment and use $\beta = 1$. We vary the size the anchor set $\mathcal{I}$ from the list $[64,128,256,512,1024]$. Fig.~\ref{fig:cmd_size} shows that the average stage performance benefits from the increase in the size of the anchor set initially. There is no significant improvement in the average stage performance when the size of the anchor set reach 128. One possible reason for this is that a randomly sampled set of size 128 is enough to provide a good estimate of the distribution of previous data in the OBGN-arxiv dataset. Therefore, increasing the size of the anchor set does not bring extra benefits and this is the reason we picked 128 for all other experiments. In addition, we expect similar property (effective size of anchor set being small) would be observed for other graph datasets because of the power law property of graph data.
