# Supplementary material for: On the Limitation and Experience Replay for GNNs in Continual Learning
Source: arXiv:2302.03534 source file (2024-07-09)
Supplement: Supplementary file 2 [file appendix_experience_replay.tex]

\section{Procedure for Solving Eq.~\eqref{eq:experience_buff}}
First recall that the optimization we want to solve is as follows.
\begin{equation}\label{eq:experience_buff}
    \begin{split}
        \min_{P_j \subset \mathcal{V}_j} \max_{u \in \mathcal{V}_j \backslash P_j} \min_{v \in P_j} d_{\text{spd}}(u,v) \quad s.t. |P_j|  = b.
    \end{split}
\end{equation}
$d_{\text{spd}}(.)$ is the shortest path distance and $b$ is the number of samples (experience) to select from each task.  Eq.~\ref{eq:experience_buff} amounts to the well-known k-center problem~\cite{approx} in graph theory and is NP-hard. For our experiment, we use Eq.~\ref{eq:experience_buff} as guidance and modify the simple greedy algorithm, farthest-first traversal, to be a sampling method for obtaining replay samples for a given task. We now describe how we modified the standard greedy algorithm into a sampling algorithm. We start with describing the standard greedy algorithm.

\begin{algorithm}[!h]
  \caption{k-center Greedy}
  \label{alg:k-center}
\begin{algorithmic}
  \REQUIRE $\mathcal{V}$ //vertex set of a given graph\\
  \REQUIRE $b$ //number of centers\\
  
  Initialize an empty array $V$
  \begin{enumerate}
     \item randomly picks a random vertex $v$ to $V$
      \item pick the next vertex to be the vertex furthest away from $V$
      \item repeat until $|V| = b$
  \end{enumerate}
\end{algorithmic}
\end{algorithm}

The procedure described above is a standard 2-approximation greedy algorithm for k-center problem. Next, we describe its sampling variant which use the distance as the chance of being sampled.

\begin{algorithm}[!h]
  \caption{Sampling for Experience Buffer}
  \label{alg:coverage_based_sampling}
\begin{algorithmic}
  \REQUIRE $\mathcal{V}_i$ //vertex set of a given graph\\
   \REQUIRE $\mathcal{G}$ //latest graph\\
  \REQUIRE $b$ //size of set to be sampled\\

  Sample/select the set of size $b$ with the following procedures:
  \begin{enumerate}
     \item initialize $P_i$ with the vertex of the highest degree.
      \item sample $u$ from $\mathcal{V}_i\backslash P_i$ based on probability $p_u$ proportion to $D_s(u,\vertexSet_i\backslash P_i) = \min_{v \in P_i}d_s(u,v)$, following the formula,
      $$p_u = \frac{D_{s}(u,P_i)}{\sum_{v \in \vertexSet_i \backslash P_i}D_{s}(v,P_i)}$$
      \item repeat until $b$ vertices are sampled
  \end{enumerate}
\end{algorithmic}
\end{algorithm}

\subsection{Running Time Complexity}
It is obvious that the procedure above runs in $\mathcal{O}(k)$ if the distance between any pair of vertices is given and runs in $\mathcal{O}(kn)$  if the distance needed to be computed for each step, where $n$ is the number of vertice of the given task.
