# Supplementary material for: On the Limitation and Experience Replay for GNNs in Continual Learning
Source: arXiv:2302.03534 source file (2024-07-09)
Supplement: Supplementary file 3 [file appendix_generalization_bound.tex]

\section{Proof of Theorem~\ref{thm:forget_bound}}\label{appendx:bound_proof}
In this appendix, we provide a proof for Theorem~\ref{thm:forget_bound}.

\begin{proof}

 Let $h^*$ denote the optimal classifier in the hypothesis space $\tilde{\mathcal{H}}$ for $\tilde{P}$ and $\tilde{P_1^2}$, i.e., 
 $$h^*= \argmin_{h \in \tilde{\mathcal{H}}} [R_{\tilde{P}}^{l'}(h) + R_{\tilde{P_1^{2}}}^{l'}(h)],$$ where $\tilde{P}$ is the induced mixed distributions of $P_1^{1}$ and $P_2^{2}$. Let $\mathcal{R}_{h_j} \Delta \mathcal{R}_{h_i}$ denote the difference (elements of different labels) between classifier $h_i$ and $h_j$ in the latent space $\mathcal{R}$. Then, for any $h \in 
 \tilde{\mathcal{H}}$ we have that 
 
 \begin{equation}\label{eq:bound}
     \begin{split}
         R_{\tilde{P_1^{2}}}^{l'}(h) & \leq  R_{\tilde{P_1^{2}}}^{l'}(h^*) + Pr_{\tilde{P_1^{2}}}(\mathcal{R}_{h} \Delta \mathcal{R}_{h^*})\\
         & \leq  R_{\tilde{P_1^{2}}}^{l'}(h^*) + Pr_{\tilde{P}}(\mathcal{R}_{h} \Delta \mathcal{R}_{h^*}) + | Pr_{\tilde{P}}(\mathcal{R}_{h}  \Delta \mathcal{R}_{h^*}) - Pr_{\tilde{P_1^{2}}}(\mathcal{R}_{h} \Delta \mathcal{R}_{h^*}) | \\
         & \leq R_{\tilde{P_1^{2}}}^{l'}(h^*) + Pr_{\tilde{P}}(\mathcal{R}_{h} \Delta \mathcal{R}_{h^*}) + d_{\tilde{\mathcal{H}} \Delta \tilde{\mathcal{H}}}(\tilde{P_1^{2}},\tilde{P})\\
         & \leq R_{\tilde{P_1^{2}}}^{l'}(h^*) + R_{\tilde{P}}^{l'}(h^*) +  R_{\tilde{P}}^{l'}(h) +  d_{\tilde{\mathcal{H}} \Delta \tilde{\mathcal{H}}}(\tilde{P_1^{2}},\tilde{P})\\
         & \leq R_{\tilde{P}}^{l'}(h) +  d_{\tilde{\mathcal{H}} \Delta \tilde{\mathcal{H}}}(\tilde{P_1^{2}},\tilde{P}) + \lambda_{\tilde{\mathcal{H}}}(\{\tilde{P_1^{2}}, \tilde{P}\})
     \end{split}
 \end{equation}

Then, we can apply the standard Vapnik-Chervonenkis theory~\citep{vc} to bound $R_{\tilde{P}}^{l'}(h)$ with the empirical estimate $\hat{R}_{\tilde{P}}^{l'}(h)$. In other words, we have that 
\begin{equation}\label{eq:vc}
    \begin{split}
        R_{\tilde{P}}^{l'}(h) \leq \hat{R}_{\tilde{P}}^{l'}(h) + \sqrt{\frac{4}{m'}(v \log{\frac{2em'}{v}} + \log{\frac{4}{\delta}})}
    \end{split}
\end{equation}

Substitute Eq.~\eqref{eq:vc} into Eq.~\eqref{eq:bound}, we obtained the result of theorem, namely
\begin{equation}
    R_{\tilde{P_1^{2}}}^{l'}(h) \leq \hat{R}_{\tilde{P}}^{l'}(h) + \sqrt{\frac{4}{m'}(d \log{\frac{2em'}{d}} + \log{\frac{4}{\delta}})}
    +d_{\tilde{\mathcal{H}} \Delta \tilde{\mathcal{H}}}(\tilde{P_1^{2}}, \tilde{P}) + \lambda_{\tilde{\mathcal{H}}}(\{\tilde{P_1^{2}}, \tilde{P}\}).
\end{equation}

\end{proof}

% \begin{theorem}[Catastrophic Forgetting Bound]\label{thm:forget_bound}
% Given a two-stage GCL problem with distributions $P_1^{1}, P_2^{2}, P_1^{2}$ and labeling function $l$, let $\mathcal{X}$ be some domain set, and $\tilde{\mathcal{H}}$ a hypothesis class of function over $\mathcal{R} \times [0,1]$ with VC-dimension of $d$. If given access to labelled sample of $m,n$ from $P_1^{1}, P_2^{2}$ and an encoder function $\mathcal{M}: \mathcal{X} \mapsto \mathcal{R}$, let $l'$ be the induced labelling function. Then with probability at least $1-\delta$, for every $h \in \tilde{\mathcal{H}}$, we have
% $R_{\tilde{P_1^{2}}}^{l'}(h) \leq \hat{R}_{\tilde{P}}^{l'}(h) + \sqrt{\frac{4}{m'}(d \log{\frac{2em'}{d}} + \log{\frac{4}{\delta}})}
%     +d_{\tilde{\mathcal{H}} \Delta \tilde{\mathcal{H}}}(\tilde{P_1^{2}}, \tilde{P}) + \lambda_{\tilde{\mathcal{H}}}(\{\tilde{P_1^{2}}, \tilde{P}\}),$
% where $m' = m + n$, $e$ is the base of natural logarithm, $\tilde{P}$ is the induced mixed distributions of $P_1^{1}$ and $P_2^{2}$, and $\hat{R}_{\tilde{P}}^{l'}(h)$ is the empirical performance.
% \end{theorem}
