# Supplementary material for: On the Limitation and Experience Replay for GNNs in Continual Learning
Source: arXiv:2302.03534 source file (2024-07-09)
Supplement: Supplementary file 4 [file appendix_related_works.tex]

\section{Related Works}\label{appendix:related_work}
In this appendix, we present a more detailed discussion of the related works as complementary to the related work section in the main papers.

\subsection{Incremental Learning}
Incremental learning, also known as continual or lifelong learning, has garnered increased attention in recent years and has been extensively investigated for Euclidean data. For a more comprehensive review of these works, we direct readers to the surveys~\citep{cl_survey,cl_survey2,cl_nlp}. The primary challenge in incremental learning lies in addressing the catastrophic forgetting problem, which is the significant decline in the performance of a model on previous tasks after training on new tasks.

Current approaches to mitigate this problem can be broadly classified into three categories: regularization-based methods, experience-replay-based methods, and parameter-isolation-based methods. Regularization-based methods aim to preserve the performance of models on previous tasks by penalizing substantial changes in the model parameters~\citep{jung2016less,li2017learning,kirkpatrick2017overcoming,farajtabar2020orthogonal,saha2021gradient}. Parameter-isolation-based methods avert drastic alterations to the parameters crucial for previous tasks by consistently introducing new parameters for new tasks~\citep{rusu2016progressive,yoon2017lifelong,yoon2019scalable,wortsman2020supermasks,wu2019large}. Experience-replay-based methods select a set of representative data from previous tasks, which are then used to retrain the model alongside new task data, preventing forgetting~\citep{lopez2017gradient,shin2017continual,aljundi2019gradient,caccia2020online,chrysakis2020online,knoblauch2020optimal}. Given the distinctive challenges of NGIL, particularly structural shifts, these established techniques may not be directly applicable. Hence, in this study, we introduce a novel experience replay method specifically crafted for NGIL.

\subsection{Incremental Learning with Graph Neural Networks}
Recent strides in GNNs have stimulated increased exploration in GIL owing to its pragmatic relevance~\citep{wang2022lifelong,xu2020graphsail,daruna2021continual,kou2020disentangle,ahrabian2021structure,cai2022multimodal,wang2020bridging,liu2021overcoming,zhang2021hierarchical,zhou2021overcoming,carta2021catastrophic,kim2022dygrain,su2023towards}. For a detailed examination of GIL methodologies and their efficacy, we direct readers to recent reviews and benchmarks~\citep{zhang2022cglb,yuan2023continual,febrinanto2023graph}.

Studies that are closely related to this work include ~\citep{ahrabian2021structure,zhou2021overcoming,kim2022dygrain,su2023towards}. ~\citep{zhou2021overcoming} has shown the feasibility and effectiveness of the experience replay framework in addressing the catastrophic forgetting problem in NGIL. However, they focus on a transductive setting where the complete graph structure is available before training and their experience replay method has neglected the structural shift problem.  ~\citep{kim2022dygrain} further investigates the changing receptive field induced by evolving graph structures using a full-graph formulation (which does not scale well as graphs grow) and proposes an experience replay strategy based on the influence score of node representation. Meanwhile, ~\citep{ahrabian2021structure} takes into account the topological awareness of GNNs and proposes an experience buffer selection based on the node degree.

There are three key distinctions between our work and these three studies. First, as discussed in~\citep{zhang2022cglb}, both ~\citep{zhou2021overcoming} and ~\citep{ahrabian2021structure} are restricted to a transductive setting, where the underlying graph structure is assumed to be given or independent throughout the learning process. This assumption neglects the structural shift issue of graph structure when transitioning to a new task, which requires specific treatment. As shown in~\citep{su2023towards}, structural shift induced by changing structure can seriously affect the performance of the model. Second, our proposed experience buffer selection relies on the topological awareness of GNNs and offers a theoretical guarantee that ensures consistent long-term performance. Lastly, instead of simply blending the experience buffer with the training set~\citep{ahrabian2021structure,zhou2021overcoming,kim2022dygrain}, we propose a novel replay method with importance reweighting for addressing the structural shift problem. 

Therefore, the inductive NGIL, wherein the graph evolves with the introduction of new tasks, remains relatively uncharted and demands a robust theoretical framework. 
\cite{su2023towards} provides the first formal study into the structural shift issue of inductive NGIL. Nevertheless, their research focuses on establishing a relation between structural shift and catastrophic forgetting in NGIL. Our works can be seen as an important extension and endeavours to further fill the void of theoretical studies of NGIL by presenting the first impossibility result on the learnability of the NGIL problem, highlighting the pivotal role of the structural shift.

Lastly, it is important to mention another research stream called dynamic/temporal graph learning, focusing on GNNs adept at capturing changing graph structures. A comprehensive review of this can be found in~\citep{dynamic_learning}. Dynamic graph learning aims to encapsulate the graph's temporal dynamics and persistently refine graph representations, with the entirety of past data at its disposal. Conversely, GIL grapples with the catastrophic forgetting dilemma, and previous task data is either inaccessible or restricted. In addition, during evaluations, a dynamic graph learning algorithm focuses on the latest data, whereas GIL models account for historical data as well.
