# Supplementary material for: On the Limitation and Experience Replay for GNNs in Continual Learning
Source: arXiv:2302.03534 source file (2024-07-09)
Supplement: Supplementary file 5 [file appendix_theorem1_proof.tex]

\section{Proof of Proposition~\ref{thm:performance_guarantee}}\label{appendix:trainset_proof}
In this appendix, we provide proof for Proposition~\ref{thm:performance_guarantee}. Before diving into the detailed proof, we present an outline of the structure of the proof and prove a lemma which we use in the proof of the theorem.

{\bf Outline of the proof for the thereom}
	\begin{enumerate}
        \item By the universal approximation power of neural network, so long there are enough parameters/weights, there exist a prediction head that can map the representation of the vertices to the correct label, Lemma~\ref{lemma:well_train}.
		\item This means that minimum (small) loss is achieved on the vertices in the replay buffer. Since loss function is lower bounded, then there exist a local region around each vertex in the training set that admit monotonic behavior, Lemma~\ref{lemma:local_structure}.
		\item With the distortion rate~\ref{def:distortion} in the premise of the theorem, we can infer a bound on the distance of the representation of other vertices to the training vertices, with respect to the structural distance given in the premise.
		\item Then, with the Assumption~\ref{assp:local_curvation} on the curvature of loss space, we can bound the loss of other vertices with the monotonic behavior and their distance to the training set in the loss space.
	\end{enumerate}

Before diving into the detailed proof of Theorem~\ref{thm:performance_guarantee}, we prove a lemma which we use in the proof of the theorem.

In this appendix, we provide a proof for Lemma~\ref{lemma:well_train} and Lemma~\ref{lemma:local_structure}.

\begin{lemma}\label{lemma:well_train}
 Let $\mathcal{D}$ be a given training set satisfying Assumption~\ref{assp:separability}. Let $\gnnModel$ be a GNN model with injective layer(s), and $f$ be a prediction function with sufficient weights. Then there exist a set of parameters $\theta_{\mathcal{D}}$ such that for any $\epsilon>0$ and $v \in \mathcal{D}$, we have
	$ \loss(f(\gnnModel_{\theta_{\mathcal{D}}}(v))) < \epsilon.$
\end{lemma}

The proof for Lemma~\ref{lemma:well_train} is mainly the application of the Assumption~\ref{assp:separability} and {\bf Theorem 1} in~\citep{memorization}. We start with restating the {\bf Theorem 1} in~\citep{memorization}.

\begin{theorem}\label{thm:uni_approx}
    There exists a two-layer neural network with ReLU activations and $2n+d$ weights that can represent any function on a sample of size $n$ in $d$ dimensions.
\end{theorem}

The proof of Theorem~\ref{thm:uni_approx} can be found in~\cite{memorization}. Other universal approximation theorem can be used to replace Theorem~\ref{thm:uni_approx}. 

\begin{proof}
  Let $\mathcal{D}$ be the training set of size $n$. By Assumption~\ref{assp:separability}, we know there is no identical inputs to the GNN in the training set. By the injective property assumed on the GNN layers, the learnt representation for all the vertex in the training are different. In other word, $\forall v, u \in \mathcal{D}$, we have that $h_u \neq h_v \in \mathds{R}^d$, where $d$ is the dimension of the embedding space. Let $\mathcal{H}_{\mathcal{D}}$ be the set of representation of the training set. It is easy to construct a mapping function $g$ that take each representation in $\mathcal{H}_{\mathcal{D}}$ to its corresponding label. By Theorem~\ref{thm:uni_approx}, the prediction $f$ can approximate $g$ arbitrarily well with a two-layer neural network of Relu activation and $2n+d$ weights.
\end{proof}

\begin{lemma}\label{lemma:local_structure}
    Let $\gnnModel$ be a GNN model trained on the vertex set $\mathcal{D}$ with injective property. Let $f$ be a prediction function with sufficient parameters. Under Assumptions~\ref{assp:local_curvation} and~\ref{assp:separability}, there exists $\theta_{\mathcal{D}}$ such that for any $v \in \mathcal{D}$ and $h_v = \gnnModel_{\theta_{\mathcal{D}}}(v)$,  there exists $r_v > 0$ such that for vectors $h,h' \in \embdingSpace$, if
	$d(h,h_v) < d(h',h_v) < r_v$,
	then %we have
	$\loss (h) < \loss (h').$
\end{lemma}

Proof of Lemma~\ref{lemma:local_structure}.
\begin{proof}
  Let $\gnnModel$ be a GNN model with injective layer(s) and $f_i$ be prediction head function
  that satisfy properties given in Lemma~\ref{lemma:well_train}. 
  
  Namely, we have for each vertex $v \in D$ and any $\epsilon > 0$,
  $$\loss(f(h_v)) < \epsilon,$$
  where $h_v = \gnnModel(v)$. This means that $\loss(f(h_v)) \mapsto 0$ and we know that the $\loss$ function is a continuous function of range $\mathds{R}_+$. $\loss(f(h_v))$ achieves the global minimum of the loss function in the embedding space. 
    
  By Assumption~\ref{assp:local_curvation}, we know that $\frac{d}{dh}\loss (f(h_v))$ and $\frac{d^2}{d^2h}\loss (f(h_v))$ exist. This implies that 
  
  $$\frac{d}{dh}\loss (f(h_v)) = 0,$$
  
  as this is the necessary condition for $h_v$ to achieve a local minimum. Furthermore, as $\loss(f(h_v))$ also achieves the global minimum, this implies that
  
  $$\frac{d^2}{d^2h}\loss (f(h_v)) \geq 0.$$

  This means that there must exist a $r_v > 0$ such that $\forall h \in N_{r_v}(h_v) \subset \embdingSpace$, we have
  
  $$\frac{d}{dh}\loss (f(h_v)) \geq 0.$$ 
  
  For $d(h,h_v) \leq d(h',h_v) \leq r_v$, we can rewrite $h' = h + d$. Then we have,
  
  \begin{equation*}
  \begin{split}
      \loss (f(h')) =  \loss (f(h + d))\\
      \geq \loss (f(h)) + \frac{d}{dh}\loss (f(h)) \|d\|
  \end{split}
  \end{equation*}
 
 Because $ \frac{d}{dh}\loss (f(h)) \geq 0$ and $\|d\| > 0$, we have that  
 $$\loss (f(h')) > \loss (f(h)).$$
\end{proof}
\begin{lemma}\label{lemma:non_intersecting_local}
    Let $P_i$ be a given replay set. $\gnnModel$ and $f$ are the GNN model and prediction function which satisfy the property in Lemma~\ref{lemma:well_train}. Let $u, v$ be two arbitrary vertexes in $P_i$ with representations $h_u = \gnnModel(u)$ and $h_v = \gnnModel(v)$. Let $N_{r_v}(h_v)$ and $N_{r_u}(h_u)$ be the neighborhood %simple region
    given in Lemma~\ref{lemma:local_structure}. Furthermore, let $N_{r_v,+}(h_v) := \{h \in N_{r_v}(h_v)| \loss(f(h)) > 0 \}$, %\cwu{it should be $N_{r_v,+}(h_v) := \{h \in N_{r_v}(h_v)|\loss(f(h))>0 \}$?}, 
    i.e., the set whose elements have positive loss values. $N_{r_u,+}(h_u)$ is Similarly defined. Then, we have that 
    $$N_{r_u,+}(h_u) \cap N_{r_v,+}(h_v) = \emptyset.$$
\end{lemma}

\begin{proof}
    Suppose the opposite: there exists $h$ which belongs to $N_{r_u,+}(h_u)$ and  $N_{r_v,+}(h_v)$ at the same time. In other words, 
    $$ h \in  N_{r_v,+}(h_v) \cap N_{r_u,+}(h_u).$$ %\cwu{$N_{r_v,+}(h_v)\cap N_{r_u,+}(h_u)$?}
    
    By their definition, % of $N_{r_v,+}(h_v)$ and $N_{r_v,+}(h_v)$, 
    $N_{r_v,+}(h_v)$ and $N_{r_u,+}(h_u)$ are open sets. By definition of an open set, there exist $r_{h,v}$ and $r_{h,u}$ such that the neighborhood $N_{r_{h,v}}(h) \subseteq N_{r_v}(h_v)$ %\cwu{$\subseteq$?} 
    and the neighborhood $N_{r_{h,u}}(h) \subseteq N_{r_u}(h_u)$ %\cwu{$\subseteq$?}. 
    
    Let $r_h = \min\{r_{h,v}, r_{h,u}\}$. We have that neighborhood $N_{r_{h}}(h)$ are in both $N_{r_u}(h_u)$ and $N_{r_v}(h_v)$.
    
    Consider $h' \in N_{r_{h}}(h)$ such that 
    $$d(h,h_v) < d(h',h_v),$$ 
    and 
    $$d(h,h_u) > d(h',h_u).$$
    Such $h'$ exists because $h_v$ and $h_u$ are two distinct points in the embedding space. Next, let's consider the loss value of $h,h'$ from the perspective of $h_v$. Because 
    $$d(h,h_v) < d(h',h_v),$$ 
    by Lemma~\ref{lemma:local_structure}, we have that
    $$\loss(f(h)) < \loss(f(h')).$$
    Similarly, if consider the loss value of $h,h'$ from the perspective of $h_u$, we have that
    $$\loss(f(h)) > \loss(f(h')),$$
    because $$d(h,h_u) > d(h',h_u).$$ 
    We reach a contradiction.
\end{proof}
Lemma~\ref{lemma:non_intersecting_local} implies that each vertex can be in at most one of these neighborhoods 
at a time. Next, we provide the proof for Theorem \ref{thm:performance_guarantee}. 

\begin{proof}
Let $\mathcal{P}_i$ be the given replay buffer for task $\tau_i$. Let $\gnnModel$ be GNN model. Without loss of generality, we may assume that all the vertices in $S_i\mathcal{P}_i$ are associated with prediction function $f_i$ Lemma~\ref{lemma:well_train}.  Let $\loss$ be the loss function with range $\mathds{R}_+$. By the premise of the theorem, we have,

	\begin{equation}
    	\sum_{u \in \mathch{P}_i} \loss (f_i (\gnnModel(u)))  = \epsilon
	\end{equation}
	
Recall that $\mathcal{V}_{i-1}$ is the accumulated vertices before $\tau_i$, and  $S_i = \mathcal{V}_i \setminus \mathch{P}_i$ which is the remaining vertex from the previous tasks. $\epsilon_i =  d_g(\mathch{P}_i,S_i)$ is the aggregated feature distance between $\mathch{P}_i$ and $S_i$.
Now, let's consider the loss on the $S_i$ which can be written as:

    \begin{equation}
        \sum_{u \in S_i} \loss (f_i(\gnnModel(u)))
    \end{equation}

By premise and Lemma~\ref{lemma:local_structure},  we have that for each $u \in S_i$, there exists at least one $v \in \mathch{P}_i$ such that $\gnnModel(u) \in N_{r_v}(\gcnModel(v))$ where $N_{r_v}(\gcnModel(v))$ satisfies properties of Lemma~\ref{lemma:local_structure}. In other words, the loss function is monotonically increasing with respect to the embedding distance in $N_{r_v}(\gcnModel(v))$. 

By Lemma~\ref{lemma:non_intersecting_local}, we know that $u$ can be in only one of this neighborhoods. Let $Q: S_i \mapsto \mathch{P}_i$ be the mapping that maps vertex $u \in S_i$ to its corresponding simple neighborhood that is centered at a vertex $Q(u) \in P_i\mathch{P}_i$. For simplicity, we denote the vertex as $q_u = Q(u)$.  Due to Lemma~\ref{lemma:local_structure} and Assumption~\ref{assp:local_curvation}, we can do a quadratic approximation of $u$ around $q_u$ and have the following upper bound:

\begin{equation}\label{eq:quadratic_approximation}
\begin{split}
        \loss (f(\gnnModel(u))) & \leq  \loss (f(\gnnModel(q_u)))+ \langle \gnnModel(u)-\gnnModel(q_u), D \gnnModel(q_u) \rangle
         + \frac{M_{u}}{2}\|\gnnModel(u)-\gnnModel(q_u)\|^2 \\
\end{split}
\end{equation}

where $M_u = \sup \{ D^2 \loss(f(h))| h \in N_{r_{q_u}}(q_u)  \},$
and
$r_{q_u} = \|q_u - u\|.$

By Assumption~\ref{assp:local_curvation}, we have that there exist $M^* >  M^*_{P_i} = \max \{ \|M_u\| | u \in T_i \}$ 
   
Then, we obtain the following upper bound that is universal for all vertexes in $S_i$: 

\begin{equation} \label{eq:upper}
    \loss (f(\gnnModel(u))) \leq  L_1(u) + \frac{M^*}{2}\|\gnnModel(u)-\gnnModel(q_u)\|^2
\end{equation}

where $$L_1(u) = \loss (f(\gnnModel(q_u)))+ \langle \gnnModel(u)-\gnnModel(q_u), D \gnnModel(q_u) \rangle.$$ 

% Because the number of task $k$ are finite, this means we can find a upper bound  $M^*$ such that
% $$M^* = \max \{M^*_{P_i} | i \in 1,..., k \}.$$

% This means that for all task $\tau_i$ we have that

% \begin{equation} \label{eq:upper}
% %     \sum_{u \in T_i} \loss (f(\gnnModel(u))) \leq \sum_{u \in T_i} L_1(u) + \frac{M^*}{2}\|\gnnModel(u)-\gnnModel(q_u)\|
% % \end{equation}

To simplify the notation, let's denote 
$$S =  \|\gnnModel(u_i)-\gnnModel(q_{u_i})\|$$

Recall that $\epsilon_i =  d_g(\mathch{P}_i,S_i)$ is the maximum graph coverage distance between $\mathch{P}_i$ and $S_i$. By Definition~\ref{def:distortion}, we have that
$$ S^2 \leq  \alpha^2 r^2 \epsilon_i^2.$$

Substitute this in Eq.~\eqref{eq:upper} and simplify the notations, we get 

\begin{equation} 
     \loss (f(\gnnModel(u))) \leq L_1(u) + \frac{M^*}{2} \alpha^2 r^2 \epsilon_i^2
\end{equation}

Since $M^*$ is bounded by Asssumption~\ref{assp:local_curvation}, we get

\begin{equation} 
    \loss_c (u) \leq \loss_c(\mathch{P}_i) + O (\alpha^2 r^2 \epsilon_i^2)
\end{equation}

This completes the proof for Theorem \ref{thm:performance_guarantee}.

\end{proof}
