# Supplementary material for: On the Limitation and Experience Replay for GNNs in Continual Learning
Source: arXiv:2302.03534 source file (2024-07-09)
Supplement: Supplementary file 6 [file appendixA.tex]

In this appendix, we provide a proof for Lemma~\ref{lemma:well_train} and Lemma~\ref{lemma:local_structure}.

\begin{lemma}\label{lemma:well_train}
 Let $\mathcal{D}$ be a given training set satisfying Assumption~\ref{assp:separability}. Let $\gnnModel$ be a GNN model with injective layer(s), and $f$ be a prediction function with sufficient weights. Then there exist a set of parameters $\theta_{\mathcal{D}}$ such that for any $\epsilon>0$ and $v \in \mathcal{D}$, we have
	$ \loss(f(\gnnModel_{\theta_{\mathcal{D}}}(v))) < \epsilon.$
\end{lemma}

The proof for Lemma~\ref{lemma:well_train} is mainly the application of the Assumption~\ref{assp:separability} and {\bf Theorem 1} in~\citep{memorization}. We start with restating the {\bf Theorem 1} in~\citep{memorization}.

\begin{theorem}\label{thm:uni_approx}
    There exists a two-layer neural network with ReLU activations and $2n+d$ weights that can represent any function on a sample of size $n$ in $d$ dimensions.
\end{theorem}

The proof of Theorem~\ref{thm:uni_approx} can be found in~\cite{memorization}. Other universal approximation theorem can be used to replace Theorem~\ref{thm:uni_approx}. 

\begin{proof}
  Let $\mathcal{D}$ be the training set of size $n$. By Assumption~\ref{assp:separability}, we know there is no identical inputs to the GNN in the training set. By the injective property assumed on the GNN layers, the learnt representation for all the vertex in the training are different. In other word, $\forall v, u \in \mathcal{D}$, we have that $h_u \neq h_v \in \mathds{R}^d$, where $d$ is the dimension of the embedding space. Let $\mathcal{H}_{\mathcal{D}}$ be the set of representation of the training set. It is easy to construct a mapping function $g$ that take each representation in $\mathcal{H}_{\mathcal{D}}$ to its corresponding label. By Theorem~\ref{thm:uni_approx}, the prediction $f$ can approximate $g$ arbitrarily well with a two-layer neural network of Relu activation and $2n+d$ weights.
\end{proof}

\begin{lemma}\label{lemma:local_structure}
    Let $\gnnModel$ be a GNN model trained on the vertex set $\mathcal{D}$ with injective property. Let $f$ be a prediction function with sufficient parameters. Under Assumptions~\ref{assp:local_curvation} and~\ref{assp:separability}, there exists $\theta_{\mathcal{D}}$ such that for any $v \in \mathcal{D}$ and $h_v = \gnnModel_{\theta_{\mathcal{D}}}(v)$,  there exists $r_v > 0$ such that for vectors $h,h' \in \embdingSpace$, if
	$d(h,h_v) < d(h',h_v) < r_v$,
	then %we have
	$\loss (h) < \loss (h').$
\end{lemma}

Proof of Lemma~\ref{lemma:local_structure}.
\begin{proof}
  Let $\gnnModel$ be a GNN model with injective layer(s) and $f_i$ be prediction head function
  that satisfy properties given in Lemma~\ref{lemma:well_train}. 
  
  Namely, we have for each vertex $v \in D$ and any $\epsilon > 0$,
  $$\loss(f(h_v)) < \epsilon,$$
  where $h_v = \gnnModel(v)$. This means that $\loss(f(h_v)) \mapsto 0$ and we know that the $\loss$ function is a continuous function of range $\mathds{R}_+$. $\loss(f(h_v))$ achieves the global minimum of the loss function in the embedding space. 
    
  By Assumption~\ref{assp:local_curvation}, we know that $\frac{d}{dh}\loss (f(h_v))$ and $\frac{d^2}{d^2h}\loss (f(h_v))$ exist. This implies that 
  
  $$\frac{d}{dh}\loss (f(h_v)) = 0,$$
  
  as this is the necessary condition for $h_v$ to achieve a local minimum. Furthermore, as $\loss(f(h_v))$ also achieves the global minimum, this implies that
  
  $$\frac{d^2}{d^2h}\loss (f(h_v)) \geq 0.$$

  This means that there must exist a $r_v > 0$ such that $\forall h \in N_{r_v}(h_v) \subset \embdingSpace$, we have
  
  $$\frac{d}{dh}\loss (f(h_v)) \geq 0.$$ 
  
  For $d(h,h_v) \leq d(h',h_v) \leq r_v$, we can rewrite $h' = h + d$. Then we have,
  
  \begin{equation*}
  \begin{split}
      \loss (f(h')) =  \loss (f(h + d))\\
      \geq \loss (f(h)) + \frac{d}{dh}\loss (f(h)) \|d\|
  \end{split}
  \end{equation*}
 
 Because $ \frac{d}{dh}\loss (f(h)) \geq 0$ and $\|d\| > 0$, we have that  
 $$\loss (f(h')) > \loss (f(h)).$$
\end{proof}
