# Supplementary material for: On the Limitation and Experience Replay for GNNs in Continual Learning
Source: arXiv:2302.03534 source file (2024-07-09)
Supplement: Supplementary file 7 [file appendix_experiments.tex]

\section{Additional Experimental Details}\label{appendx:exp}
In this appendix, we provide additional experimental results and a detailed set-up of the experiments for reproducibility.

\subsection{Optimization Methods}
For all our experiments, we use Adam optimization method~\citep{adam} with a learning rate of 1e-2, weight decay of 5e-4 and zero drop-out. All the experiments are trained on a single GPU with default epoch number of 100 and batch size of 1024.

\subsection{Detailed Dataset Description}
For our experiments, we used the following real-world datasets, Cora and OGBN-arxiv, provided by DGL~\citep{dgl}. Both Cora and OGBN-arxiv are citation networks where the node represents paper and the edge represents citation relation. In addition, OGBN-arxiv has an additional attribute on the year when the paper was published. This allows for a natural partition of the learning stage for the experiment. Nodes in the graph are anonymized and do not contain any personally identifiable data. Table~\ref{tab:data_description} gives a more detailed description of the statistic of the two datasets. 

\begin{table*}[!h]
  \centering
  \caption{Description on the datasets
  }  
  
  {\small
   \setlength\tabcolsep{4pt}
    \begin{tabular}{c|cc}
    \toprule
        Datasets  &        Cora   & OGB-Arxiv          \\
            
    \midrule
          Number of Vertexes & 2,708 & 169,343\\
          Number of Edges   & 10,556 & 1,166,243	\\
          Dimension of Node Feature & 1,433 & 128 \\
         Number of Class & 7 & 40\\
    \bottomrule
    \end{tabular}%
    
   }
  \label{tab:data_description}%
\end{table*}%

For Cora, we use the default train/valid/test split provided by the library for the static setting. To create a continual setting for Cora, we first extract the largest component of the Cora dataset (which makes up most of the dataset) and then apply the fluid community detection algorithm~\citep{fluid} provided by NetworkX. Two communities are resulted from the fluid community detection algorithm and we randomly assign each community to stage 1 or 2. To create a training/valid set for each stage, we randomly pick 10\% (which is roughly the same ratio as the provided training set) of the labelled data as the training set and pick another 10\% of labelled data as the validation set. Then, we use the rest of the data as the test set. 

For OGBN-arxiv, we use the default train/valid/test split provided by the library for the static setting. However, to keep the experiments consistent, we randomly pick a subset of size 17000 (roughly 10 \% of the dataset) from the default training set as the new training set. For the continual setting, we partition the vertices naturally by their timestamps. Especially, we use three stages: stage 1 consists of papers published until 2017, stage 2 consists of papers published in 2017-2018, and stage 3 consists of papers published after 2018. For each stage, we randomly pick 10 \% of the stage data as the training set and another 10 \% as the validation set. Then, we use the rest of the data from each stage as the test set for that stage.

\subsection{Contextual Stochastic Block Model}
We use the contextual stochastic block model~\citep{cSBM} to create a graph for each learning stage. For each graph, we create 300 vertices and assign them a community label $\{0,1\}$. We refer to a specific ratio of vertices from different communities as a configuration and the formula we use to vary the community ratio is as follows, configuration $i = (150+(i-1)*25,150-(i-1)*25,150-(i-1)*25,150+(i-1)*25)$. As $i$ increases, the difference in the ratio of the two learning stages increases. Intuitively, this should allow us to control the distribution difference between different learning stages.

Then we follow the standard stochastic block model. We use $p_{intra} = 0.15$ to randomly create edges among vertices of the same community and $p_{inter} = 0.1$ to randomly create edges among vertices of different communities. Then, we use $p_{stage} = [0.025,0.05,0.08,0.1,0.15]$ to create edges among vertices of different learning stages.

Then, the node features $x_v$ of each vertex is created based on the following formula,
$$x_v = \sqrt{\frac{\mu}{n}} y_v u + \frac{Z_v}{p},$$
where $y_v \in \{0,1\}$ is the community label of vertex $v$,  $u, Z_v \sim \mathcal{N}(0, I)$ are random Gaussian of dimension $p$, $n$ is the number of vertices in the graph and $\mu$ is a hyper-parameter of the model to control how separable of the features of the vertices from different communities. For our experiments, we use $\mu=5, n=300, p=500$ for graph in each stage. 

\subsection{Graph Neural Network Details}
For our experiments, we use two popular GNN models, GCN~\citep{gcn} and GraphSage~\citep{sage}. For implementation, we use the default implementation provided by DGL for realizing these models. For all our experiments, we use two GNN layers followed by an additional readout function of an MLP layer. We use Sigmoid as the activation function for the last hidden layer and Relu for the rest of the layers. We only vary the hidden dimension of the GNN layer for each experiment.
