# Supplementary material for: On the Limitation and Experience Replay for GNNs in Continual Learning
Source: arXiv:2302.03534 source file (2024-07-09)
Supplement: Supplementary file 10 [file appendix_expressiveness_sample.tex]

\section{Additional Discussion and Results on Expressiveness and Sample Complexity}
